# Supplementary material for: OpenIns3D: Snap and Lookup for 3D Open-vocabulary Instance Segmentation
Source: arXiv:2309.00616 source file (2024-08-12)
Supplement: Supplementary file 1 [file 2d-input-free.tex]

\begin{figure*}[h!]
 \centering
 \includegraphics[width=1.0\textwidth]{figs_appendix/2d-input-free.pdf}
 \centering
\caption{\textbf{Comparison of the OpenIns3D framework with other models.} OpenIns3D offers a unique capability of using only 3D input, making it more applicable in real-life scenarios.
a) 3D feature distillation frameworks, where 2D images are used as a bridge to distill language-aligned features into 3D, with typical works including OpenScene \citep{peng2022openscene} and Clip2Scene \citep{chen2023clip2scene}.
b) Building 3D-text pairs, where 2D captioning models are used to build 3D-text pairs for feature learning, with typical works including PLA-family \citep{ding2023lowis3d, yang2023regionplc, ding2022language}.
c) CLIP and Projection, where objects are cropped out of 2D images before being processed by CLIP, and the results are directly projected into 3D, including OpenMask3D \citep{takmaz2023openmask3d} and OV-3DET \citep{lu2023open}. d) Mask-Snap-lookup, where only 3D input is needed for 3d open world scene understanding tasks}

 \label{fig: 2d-input-free}
\end{figure*}
